# Supplementary material for: Justin: Hybrid CPU/Memory Elastic Scaling for Distributed Stream Processing
Source: arXiv:2505.19739 source file (2025-05-26)
Supplement: Supplementary file 1 [file appendix.tex]

\newpage
\appendix
\section{Artifact}
\subsection{Claims}
We provide the source-code of \sysname, as well as deployment scripts and notebooks to reproduce the results presented in the paper.
The GitHub repository \url{https://github.com/CloudLargeScale-UCLouvain/flink-justin} contains the available code, which will be later made available on Zenodo\ds{Include URL}.

We make the following functionality claims:
\begin{itemize}
    \item \textbf{F1:} The microbenchmarks presented in Section~\ref{sec:motivations}~(Figure~\ref{fig:microbenchmarks}) showing the impact of memory allocation on state access performance using RocksDB can be reproduced through this artifact.
    \item \textbf{F2:} The results obtained in Section~\ref{sec:eval:results}~(Figure~\ref{fig:nexmark}) showing an improvement of the state-of-the-art autoscaler by enabling heterogeneous resource allocations can be reproduced through this artifact.
\end{itemize}

Finally, we make the following reusability claims:
\begin{itemize}
    \item \textbf{R1:} \sysname triggers automatic scaling decisions on any queries, not solely the ones used for this paper evaluation.
    \item \textbf{R2:} New policies can be easily integrated into \sysname as long as their final output is a scaling configuration (cf. Section~\ref{sec:justin}).
    \item \textbf{R3:} \sysname policy thresholds can be easily modified and at runtime, to further enable smart scaling decisions (cf. Section~\ref{sec:evaluation}).
\end{itemize}
\subsection{Setup}
\mypara{Infrastructure}
We include setup scripts for both local, using Kind, and remote executions, using the Grid5000.
Guest accounts can be requested following this web page: \url{https://www.grid5000.fr/w/Grid5000:Get_an_account}.

Notebooks located in the folder \texttt{scripts/infra/\{g5k, kind\}} create the clusters and install the required tools.
You will need the required \url{https://kubernetes.io/docs/reference/kubectl/} and \url{https://helm.sh/docs/helm/helm_install/} binaries, depending on your architecture, and put them in the \texttt{scripts/tools} folder.

The experiments were conducted on Grid5000 and we thus strongly recommend using this setup, as the Kind deployment creates virtual nodes in the form of Docker containers instead of using multiple machines.\\
The file \texttt{scripts/infra/g5k/main.tf} contains the Grid5000 reservation. 
We recommend using either the \emph{Ecotype} cluster on the Nantes site or the \emph{Gros} cluster in Nancy.
We also recommend book at least 7 nodes for a duration of 3 hours minimum.
You can initialize the cluster by running the full \texttt{init-cluster.ipynb} notebook.

\mypara{Compiling \sysname}
To setup \sysname, you will need to compile the following Maven projects:
\begin{itemize}
    \item \textbf{Flink Kubernetes Operator}: head to the flink-kubernetes-operator folder and build the Docker image with:\\
    \texttt{docker build . -t DOCKER\_ID/flink-kubernetes-operator:dais}\\
    \texttt{docker push DOCKER\_ID/flink-kubernetes-operator:dais}\\
    Next, we need to deploy the operator using Helm.
    Head to the \texttt{scripts} folder and execute:\\
    \texttt{export DOCKER\_ID=...; ./deploy\_operator.sh}\\
    Make sure to replace your DOCKER\_ID in the previous command.
    \item \textbf{Benchmarks}: compiling the benchmarks before Flink is necessary to include the Jars into the Flink image.
    Head to the \texttt{benchmarks} folder and execute:\\
    \texttt{mvn clean package}\\
    \item \textbf{Flink}: head to the \texttt{script} folder and execute the following commands:\\
    \texttt{export DOCKER\_ID=...; ./compile\_flink.sh}\\
    The script will compile Flink (takes a couple minutes), then build and push the Docker image.
    Make sure to replace your DOCKER\_ID in the previous command.
\end{itemize}

\subsection{Execution}
The experiments conducted to generate Figure~\ref{fig:microbenchmarks} (\textbf{F1}) are located in the folder \texttt{notebooks/motivation}.
The notebook will execute each configuration of each query for 10 minutes.
The duration of an experiment can be lowered by reducing the sleep time in the corresponding cells.
The metrics are available on Prometheus through Grafana, as explained in the last cell.

Finally, the macro-benchmark queries used in Figure\ref{fig:nexmark} (\textbf{F2}) are located in the folder \texttt{notebooks/nexmark}.
Each query must be executed twice, once with the default auto-scaler enabled, by setting the \texttt{job.autoscaler.justin.enabled} option to \texttt{false}, and once using \sysname by enabling the option.

\subsection{Playing with the artifact}

\sysname is compatible with any \flink Query (\textbf{R1}).
The only requirement is for the query to include jar dependencies (e.g. Flink Streaming API) when submitted.

We integrated the \sysname policy into the Flink Kubernetes Operator, more precisely in the \texttt{ScalingExecutor.java} class of the \texttt{org.apache.flink.autoscaler} package.
This policy can be modified by the reader to reflect another algorithm then the one proposed in Algorithm~\ref{alg:policy} (\textbf{R2}).
The reader would need to re-build the docker image of the operator and re-deploy it.

Finally, the policy thresholds are parameterized inside each query YAML configuration file and can be modified to trigger different scaling decisions than the ones presented in the evaluation (\textbf{R3}).
